# Supplementary material for: Learning Decision Policies with Instrumental Variables through Double Machine Learning
Source: arXiv:2405.08498 source file (2024-06-28)
Supplement: Supplementary file 1 [file appendix.tex]

\section{Broader Impact and Limitations}
In many safety-critical applications, one needs to infer causal structure from observational data e.g. in healthcare, economics, or geosciences since interventions are unethical or simply impossible. For these cases, one requires algorithms that have theoretical guarantees, are robust to hidden confounding, and are computationally efficient. We hope that in the long term, our work can thus contribute to better machine learning-driven decision-making in safety-critical environments. 

While theoretical guarantees and extensive experiments are critical components for the evaluation of algorithms, especially in safety-critical environments this can potentially lead to a false sense of security and trust. Constant monitoring and assessment by domain experts are needed before and during the deployment of any machine learning algorithm, especially in safety-critical environments.  

One key limitation of our approach as well as of all causal discovery approaches from observational data is the reliance on additional assumptions. These assumptions are required since causal discovery from observational data is impossible without them.  We related our assumptions to previous ones in the Framework Section $\ref{sec:framework}$. These assumptions of our approach need to be checked before applying the approach but are less restrictive than for comparable baselines. Moreover, since our approach is inspired by debiased machine learning, the focus is on inferring the true or "debiased" underlying structure rather than obtaining low variance estimates of the structure. 

%Since our work is inspired by debiased machine learning approaches the focus of this work is on obtaining true, causal or unbiased estimates rather than ones which low variance. 

\section{Direct Causal Effects and Interventions}
\label{app:interventions}
In this section, we clarify the notion of an intervention and direct causal effects. We will also introduce some notation that will be used later on in the proofs.

We consider interventions by which a random variable $X^j_t$ is set to a constant $X^j_t \gets x$. We denote with $Y_{T} \mid do(X^i_t = x)$ the outcome time series $\boldsymbol{Y}$ at time step $T$, after performing an intervention as described above. We can likewise perform multiple joint interventions, by setting a group of random variables $\boldsymbol I $ at different time steps, to pre-determined constants specified by an array $\boldsymbol i$. We use the symbol $Y_T \mid do(\boldsymbol I = \boldsymbol i)$ to denote the resulting post-interventional outcome, and we denote with $\pr{Y_T = y \mid do(\boldsymbol I = \boldsymbol i)}$ the probability of the event $\{Y_T \mid do(\boldsymbol I = \boldsymbol i) = y\}$.

Using this notation, a time series $\boldsymbol{X}^i$ has a direct effect on the outcome $\boldsymbol{Y}$, if performing different interventions on the variables $\boldsymbol{X}^i$, while keeping the remaining variables fixed, will alter the probability distribution of the outcome $\boldsymbol{Y}$. Formally, define the sets of random variables $\boldsymbol{I}_{T}\coloneqq \{X_{t}^1, \dots, X_{t}^n , Y_t\}_{ t < T}$, which consists of all the information before time step $T$. Similarly, define the random variable $\boldsymbol{X}^i_T \coloneqq \{X^i_t\}_{t < T}$, consisting of all the information of time series $\boldsymbol{X}^i$ before time step $T$. Define the variable $\boldsymbol{I}_{T}^{\setminus i}\coloneqq \boldsymbol{I}_{T} \setminus \boldsymbol{X}^i_T$, which consists of all the variables in $\boldsymbol{I}_T$ except for $\boldsymbol{X}^i_T$. Then, a time series $\boldsymbol{X}^i$ has a direct effect on the outcome $ \boldsymbol{Y}$ if it holds
\begin{equation}
\label{eq:direct_effect}   
\pr {Y_T = y \mid do \left (\boldsymbol{X}^i_T = \boldsymbol{x}' , \boldsymbol{I}_{T}^{\setminus i} =  \boldsymbol{i} \right )} \neq \pr {Y_T = y \mid do \left (\boldsymbol{X}^i_T = \boldsymbol{x}'' , \boldsymbol{I}_{T}^{\setminus i} =  \boldsymbol{i} \right )}
\end{equation}
We say that a time series $\boldsymbol{X}^i$ causes $\boldsymbol{Y}$, if there is a direct effect between $\boldsymbol{X}^i$ and $\boldsymbol{Y}$ as in Eq. \ref{eq:direct_effect}, for any time step $T$.
%
%Following, e.g., \cite{DBLP:conf/icml/MastakouriSJ21}, we define the \emph{full time} graph $\mathcal{G}$ as a directed graph whose edges represent all direct causal effects among the variables at all time steps. Given the outcome $Y_T$ at a given time step, we refer to the parent nodes in the full-time graph as its \emph{causal parents}. We further define the \emph{summary} graph whose nodes are $\boldsymbol{X}^i$ and $\boldsymbol{Y}$, and with directed edges representing causal effects between the time series. We refer the reader to Figure \ref{fig:graph} for a visualization of these graphs. Note that the causes of $\boldsymbol{Y}$ correspond to the parent nodes of $\boldsymbol{Y}$ in the summary graph.
%
\section{Necessity of the Statistical Independence of $\varepsilon_t$}
\label{sec:counterexample}
We provide a counterexample, to show that if there are dependencies between the noise and the historical data, then the causal structure may not be identifiable from observational data. To this end, we consider a first dataset $\{X_t, Y_t\}_{t \in \mathbb{Z}}$, defined as
\begin{equation*}
%\left \{
%\begin{array}{l}
%X_t = N_{t-1} \\
%Y_t = \varepsilon_t
%\end{array}
%\right .
%\quad \text{with} \quad 
\begin{array}{l}
X_{t-1}, Y_t \sim \mathcal{N}(\boldsymbol 0, \Sigma) %\ \text{for} \ t \geq 0 \\
%Y_0 = \varepsilon_0
\end{array}
\end{equation*}
Here, $\mathcal{N}(\boldsymbol 0, \Sigma)$ is a zero-mean joint Gaussian distribution with covariance matrix
\begin{equation*}
\Sigma = \left [
\begin{array}{cc}
1 & 1 \\
1 & 1
\end{array}
\right ].
\end{equation*}
We also consider a second dataset $\{W_t, Z_t\}_{t \in \mathbb{Z}}$, defined as 
\begin{equation*}
W_t \sim \mathcal{N}(0, 1), \quad Z_t = W_{t-1} %\left \{
%\begin{array}{l}
%W_t = W_{t-1} \\
%Z_t = Z_{t-1} + W_{t-1} + \varepsilon_t
%\end{array}
%\right .
%\quad \text{with} \quad 
%\begin{array}{l}
%W_0, \varepsilon_0 \sim \mathcal{N}(\boldsymbol 0, \Sigma) \\
%Z_0 = \varepsilon_0 \\
%\varepsilon_t \equiv 0 \ %\text{for}\  t > 0
%\end{array}
\end{equation*}
The parameter $\Sigma$ is defined as above. Both datasets entail the same joint probability distribution. However, the causal diagrams change from one dataset to the other. Hence, the causal structure cannot be recovered from observational data, if the posterior additive noise $\varepsilon_t$ is correlated with some of the covariates.

\section{Necessity of No Instantaneous Causal Effects\\between $\boldsymbol{Y}$ and the Potential Causes $\boldsymbol{X}^i$} \label{app:instantaneous}

Here, we provide a counterexample to show that without the no instantaneous causal effect, the causal structure may not be identifiable from observational data. Consider the following two models:

\begin{itemize}
    \item Model 1: We consider time series $\{X_t\}$, $\{Y_t\}$ of the form $X_t = \mathbb{E}[X_{t-1}] + c$ and $Y_t = \mathbb{E}[Y_{t-1}-X_{t-1}] + X_t$. In this model, $c$ is a random variable drawn from a Gaussian distribution with a mean of 0 and covariance of 1.

    \item Model 2: We consider time series $\{X_t\}$, $\{Y_t\}$ of the form $Y_t = \mathbb{E}[Y_{t-1}] + c$ and $X_t = \mathbb{E}[X_{t-1}-Y_{t-1}] + Y_t$. In this model, $c$ is a random variable drawn from a Gaussian distribution with a mean of 0 and covariance of 1.
\end{itemize}
Both models entail the same joint distribution. However, in Model 1 $X$ has a causal effect on $Y$, whereas in Model 2 $Y$ has a causal effect on $X$. Hence, in this example, the causal structure is not identifiable.

\section{Proof of Theorem \ref{thm:granger}}
\label{app:granger}
We prove the following result.
\granger*
\begin{proof}
We first prove that it holds
\begin{equation}
\label{eq:2_new}
    \pr{Y_T = y \mid do(X^i_{t} = x,\boldsymbol{I}_{T}^{\setminus i} = \boldsymbol{i})} = \pr{Y_T = y \mid X^i_{t} = x,\boldsymbol{I}_{T}^{\setminus i} = \boldsymbol{i}}
\end{equation}
for any non-zero event $\{ Y_T = y \}$. To this end, define the group $\boldsymbol{P} $ consisting of all the causal parents of the outcome. Note that $\boldsymbol{P} \subseteq \{X^i_t, \boldsymbol{I}_{T}^{\setminus i}\} $. By \ref{cond:1}, the outcome can be described as $Y = f(\boldsymbol{P}) + \varepsilon$, where $\varepsilon$ is independent of $\{X^i_t, \boldsymbol{I}_{T}^{\setminus i} \}$. Hence by Rule 2 of the do-calculus (see \cite{pearlj}, page~85) Eq. \ref{eq:2_new} holds, since $Y$ becomes independent of $\{X^i_t, \boldsymbol{I}_{T}^{\setminus i} \}$ once all arrows from $\boldsymbol{P}$ to $Y$ are removed from the graph of the DGP.

We now prove the claim using Eq. \ref{eq:2_new}. To this end, assume that Eq. \ref{eq:2_new} holds and suppose that $X^i$ does not Granger causes $Y$, i.e., it holds
\begin{equation}
\label{eq:granger}
\pr{Y_T=y\mid X^i_{t} = x,\boldsymbol{I}_{T}^{\setminus i} = \boldsymbol{i}} = \pr{Y_T=y\mid  \boldsymbol{I}_{T}^{\setminus i} = \boldsymbol{i}},
\end{equation}
for any non-zero event $\{Y_T = y\}$. Then, 
\begin{align*}
    \pr{Y_T=y\mid do(X^i_{t} = x,\boldsymbol{I}_{T}^{\setminus i} = \boldsymbol{i})} & = \pr{Y_T=y\mid X^i_{t} = x,\boldsymbol{I}_{T}^{\setminus i} = \boldsymbol{i}} & [\text{Eq. \ref{eq:2_new}}] \\
    & = \pr{Y_T=y\mid  \boldsymbol{I}_{T}^{\setminus i} = \boldsymbol{i}} & [\text{Eq. \ref{eq:granger}}] \\
    & = \pr{Y_T=y\mid X^i_{t} = x',\boldsymbol{I}_{T}^{\setminus i} = \boldsymbol{i}} & [\text{Eq. \ref{eq:granger}}] \\
    & = \pr{Y_T=y\mid do(X^i_{t} = x',\boldsymbol{I}_{T}^{\setminus i} = \boldsymbol{i})}. & [\text{Eq. \ref{eq:2_new}}]
\end{align*}
Hence, causality implies Granger causality.

We now prove that Granger causality implies causality. To this end, suppose that $X^i$ is not a potential cause of $Y$. By the definition of direct effects, it holds
\begin{align}
& \pr{Y_T=y\mid do(X^i_{t} = x,\boldsymbol{I}_{T}^{\setminus i} = \boldsymbol{i})} \nonumber \\
& \qquad \qquad \qquad = \expect{}{\pr{Y_T=y\mid do(X^i_{t} = x', \boldsymbol{I}_{T}^{\setminus i} = \boldsymbol{i})} \mid \boldsymbol{I}_{T}^{\setminus i} = \boldsymbol{i}}. \label{eq:lemma101}
\end{align}
Hence,
\begin{align*}
    & \pr{Y_T=y\mid do(X^i_{t} = x,\boldsymbol{I}_{T}^{\setminus i} = \boldsymbol{i})} & \\
    & \qquad  \qquad = \pr{Y_T=y\mid X^i_{t} = x,\boldsymbol{I}_{T}^{\setminus i} = \boldsymbol{i}} & [\text{Eq. \ref{eq:2_new}}]\\
    & \qquad  \qquad = \expect{}{\pr{Y_T=y\mid do(X^i_{t}, \boldsymbol{I}_{T}^{\setminus i})}\mid \boldsymbol{I}_{T}^{\setminus i} = \boldsymbol{i}} & [\text{Eq. \ref{eq:lemma101}}]\\
    & \qquad  \qquad = \expect{}{\pr{Y_T=y\mid X^i_{t} , \boldsymbol{I}_{T}^{\setminus i} }\mid \boldsymbol{I}_{T}^{\setminus i} = \boldsymbol{i}} & [\text{Eq. \ref{eq:2_new}}]\\
    & \qquad  \qquad = \pr{Y_T=y\mid  \boldsymbol{I}_{T}^{\setminus i} = \boldsymbol{i}}, & 
\end{align*}
and the claim follows. 
\end{proof}
\section{Proof of Theorem \ref{lemma:cond_variance}}
\label{app:cond_variance}
We prove the following result.
\cond*
In order to prove Theorem \ref{lemma:cond_variance}, we use the following auxiliary lemma.
\begin{lemma}
\label{lemma:expect}
Consider a causal model as in \ref{cond:1}-\ref{cond:3}. Then, the following conditions are equivalent:
\begin{enumerate}
    \item $\expect{}{Y_T \mid X^i_{t} = x,\boldsymbol{I}_{T}^{\setminus i} = \boldsymbol{i}} = \expect{}{Y_T \mid X^i_{t} = x', \boldsymbol{I}_{T}^{\setminus i} = \boldsymbol{i}}$  a.s. ; \label{itemone}
    \item $\pr{Y_T = y \mid X^i_{t} = x,\boldsymbol{I}_{T}^{\setminus i} = \boldsymbol{i}} = \pr{Y_T=y \mid X^i_{t} = x', \boldsymbol{I}_{T}^{\setminus i} = \boldsymbol{i}}$ a.s. \label{itemtwo}
\end{enumerate}
\end{lemma}
\begin{proof}
Clearly, Item \ref{itemtwo} implies Item \ref{itemone}. 

We now prove the converse, i.e., we show that Item \ref{itemone} implies Item \ref{itemtwo}. To this end,
define the group $\boldsymbol{P}_T $ consisting of all the causal parents of $Y_T$. Note that it holds $\boldsymbol{P}_T \subseteq \{\boldsymbol{I}_{T}^{\setminus i}, X^i_{t}\} \subseteq \{\boldsymbol{I}_{T}^{\setminus i}, X^i_{t}\}$. Hence, the joint intervention $\{ X^i_{t},\boldsymbol{i}^{i,t}_{T-1}\} \gets \{x,\boldsymbol{i}\}$ define an intervention on the parents $\boldsymbol{P}_T \gets \boldsymbol{p}$. Further, we can write the potential outcome as 
\begin{equation}
\label{eq:new_eq1}
Y_T\mid do(X^i_{t} = x,\boldsymbol{I}_{T}^{\setminus i} = \boldsymbol{i}) = f(\boldsymbol{p}) + \varepsilon . 
\end{equation}
Similarly, the joint intervention $\{X^i_{t},\boldsymbol{I}^{i,t}_{T-1}\} \gets \{x,\boldsymbol{i}\}$, define an intervention on the parents $\boldsymbol{P}_T \gets \boldsymbol{p}'$. We can write the potential outcome as 
\begin{equation}
\label{eq:new_eq2}
Y_T\mid do(X^i_{t} = x',\boldsymbol{I}_{T}^{\setminus i} = \boldsymbol{i}) = f(\boldsymbol{p}') + \varepsilon .
\end{equation}
Hence, it holds
\begin{align}
    f(\boldsymbol{p}) + \expect{}{\varepsilon} & = \expect{}{Y_T\mid do(X^i_{t} = x,\boldsymbol{I}_{T}^{\setminus i} = \boldsymbol{i})} & [\text{Eq. \ref{eq:new_eq1}}] \nonumber \\ 
    & = \expect{}{Y_T\mid X^i_{t} = x,\boldsymbol{I}_{T}^{\setminus i} = \boldsymbol{i}} & [\text{Eq. \ref{eq:2_new}, Theorem \ref{thm:granger}}] \nonumber \\ 
    & = \expect{}{Y_T\mid X^i_{t} = x',\boldsymbol{I}_{T}^{\setminus i} = \boldsymbol{i}} & [\text{by assumption}] \nonumber \\ 
    & = \expect{}{Y_T\mid do(X^i_{t} = x',\boldsymbol{I}_{T}^{\setminus i} = \boldsymbol{i})} & [\text{Eq. \ref{eq:2_new}, Theorem \ref{thm:granger}}] \nonumber \\ 
    & = f(\boldsymbol{p}')+ \expect{}{\varepsilon}.  & [\text{Eq. \ref{eq:new_eq2}}] \nonumber
\end{align}
By \ref{cond:1}, the variable $\varepsilon$ is exogenous independent noise. From the chain of equations above it follows that $f(\boldsymbol{p}) = f(\boldsymbol{p}')$. Hence, 
\begin{align}
& \pr{Y_T = y\mid do(X^i_{t} = x,\boldsymbol{I}_{T}^{\setminus i} = \boldsymbol{i})} = \pr{f(\boldsymbol{p}) + \varepsilon = y} \nonumber \\ 
& \qquad \qquad \qquad = \pr{f(\boldsymbol{p}') + \varepsilon = y} = \pr{Y_T = y\mid do(X^i_{t} = x',\boldsymbol{I}_{T}^{\setminus i} = \boldsymbol{i})} \label{eq:new_3}
\end{align}
We conclude that it holds
\begin{align*}
    & \pr{Y_T=y\mid X^i_{t} = x,\boldsymbol{I}_{T}^{\setminus i} = \boldsymbol{i}} & \\
    & \qquad = \pr{Y_T\mid do(X^i_{t} = x,\boldsymbol{I}_{T}^{\setminus i} = \boldsymbol{i})} & [\text{Eq. \ref{eq:2_new}, Theorem \ref{thm:granger}}] \\ 
    & \qquad = \pr{Y_T=y\mid do(X^i_{t} = x',\boldsymbol{I}_{T}^{\setminus i} = \boldsymbol{i})} & [\text{Eq. \ref{eq:new_3}}] \\ 
    & \qquad = \pr{Y_T=y\mid X^i_{t} = x',\boldsymbol{I}_{T}^{\setminus i} = \boldsymbol{i}}, & [\text{Eq. \ref{eq:2_new}, Theorem \ref{thm:granger}}]
\end{align*}
as claimed.
\end{proof}
We can now prove the main result.
\begin{proof}[Proof of Theorem \ref{lemma:cond_variance}]
We first prove that $X^i$ Granger causes $Y$ iff. it holds 
\begin{equation}
\label{eq:chi}
\expect{}{\left ( \expect{}{Y_T\mid X^i_{t} ,\boldsymbol{I}_{T}^{\setminus i} } - \expect{}{Y_T\mid \boldsymbol{I}_{T}^{\setminus i} } \right )^2} \neq 0.
\end{equation}

First, suppose that Eq. \ref{eq:chi} does not hold. Then, it holds $\mathbb{e}[Y_T \mid X^i_{t} = x,\boldsymbol{I}_{T}^{\setminus i} = \boldsymbol{i}] = \mathbb{E}[Y_T \mid X^i_{t} = x',\boldsymbol{I}_{T}^{\setminus i} = \boldsymbol{i}]$, a.s. Combining this equation with Lemma \ref{lemma:expect} yields
\begin{align*}
    \pr{Y_T = y \mid X^i_{t} = x,\boldsymbol{I}_{T}^{\setminus i} = \boldsymbol{i}} & = \expect{}{\pr{Y_T = y \mid X^i_{t} ,\boldsymbol{I}_{T}^{\setminus i} } \mid \boldsymbol{I}_{T}^{\setminus i} = \boldsymbol{i}}\\
    & = \pr{Y_T = y \mid \boldsymbol{I}_{T}^{\setminus i} = \boldsymbol{i}},
\end{align*}
a.s. Hence, if $X^i$ Granger causes $Y$, then Eq. \ref{eq:chi} holds.
\begin{align}
\label{eq:chi2}
    \expect{}{Y_T \mid X^i_{t} = x,\boldsymbol{I}_{T}^{\setminus i} = \boldsymbol{i}} \neq \expect{}{Y_T \mid X^i_{t} = x',\boldsymbol{I}_{T}^{\setminus i} = \boldsymbol{i}},
\end{align}
for a triple $\{x, x', \mathbf{w} \}$. By combining Eq. \ref{eq:chi2} with Lemma \ref{lemma:expect} we see that Eq. \ref{eq:chi} implies causality. However, by Theorem \ref{thm:granger} Granger causality is equivalent to causality in this case.

We now prove the claim. By the tower property of the expectation~\cite{Williams-1991} that
\begin{align*}
    & \expect{}{\left ( \expect{}{Y_T\mid X^i_{t},\boldsymbol{I}_{T}^{\setminus i}} - \expect{}{Y_T\mid \boldsymbol{I}_{T}^{\setminus i}} \right )^2} \\
    & =  \expect{}{\left (\expect{}{Y_T\mid X^i_{t},\boldsymbol{I}_{T}^{\setminus i}} - \expect{}{Y_T\mid \boldsymbol{I}_{T}^{\setminus i}} \right )^2} \\
    & = \expect{}{\expect{}{\left (\expect{}{Y_T\mid X^i_{t},\boldsymbol{I}_{T}^{\setminus i}} - \expect{}{Y_T\mid \boldsymbol{I}_{T}^{\setminus i}} \right )^2\mid \boldsymbol{I}_{T}^{\setminus i}}} \\
    & = \expect{}{\expect{}{\left (\expect{}{Y_T\mid X^i_{t},\boldsymbol{I}_{T}^{\setminus i}}^2 - \expect{}{Y_T\mid X^i_{t},\boldsymbol{I}_{T}^{\setminus i}}  \expect{}{Y_T\mid \boldsymbol{I}_{T}^{\setminus i}} \right )\mid \boldsymbol{I}_{T}^{\setminus i}}} \\
    & = \expect{}{\expect{}{Y_T\mid X^i_{t},\boldsymbol{I}_{T}^{\setminus i}}^2} - \expect{}{\expect{}{\left (\expect{}{Y_T\mid X^i_{t},\boldsymbol{I}_{T}^{\setminus i}}  \expect{}{Y_T\mid \boldsymbol{I}_{T}^{\setminus i}}\right )\mid \boldsymbol{I}_{T}^{\setminus i}}}\\
    & = \expect{}{\expect{}{Y_T\mid X^i_{t},\boldsymbol{I}_{T}^{\setminus i}}^2} - \expect{}{\expect{}{Y_T\mid \boldsymbol{I}_{T}^{\setminus i}}^2}\\
    & = \expect{}{Y_T\expect{}{Y_T\mid X^i_{t},\boldsymbol{I}_{T}^{\setminus i}}} - \expect{}{Y_T\expect{}{Y_T\mid \boldsymbol{I}_{T}^{\setminus i}}},
\end{align*}
as claimed.
\end{proof}

\section{Intuition on Zero-Masking}
\label{app:zero-mask}
We provide intuition why masking is a reasonably good idea. Assume that the function $\widehat{f}$ is a $\epsilon$-close estimator of the true function $f^*$ in the $\mathcal{L}^2(P_{X_1, X_2, \dots, X_m})$ norm, where the functions $\widehat{f}, f^*$ and the joint probability distribution $P_{X_2, \dots, X_m}$ are defined on the set $\{X_1, X_2, \dots, X_m\}$,

$$ ||\widehat{f} - f^*||_{\mathcal{L}^2(P_{X_1, X_2, \dots, X_m})} \leq \epsilon$$

Now, let's mask the random variable $X_1$. We are interested to see how close is the estimator $\mathbb{E}_{X_1}\widehat{f}$ to the true function $\mathbb{E}_{X_1}f^*$ in the $\mathcal{L}^2(P_{X_2, \dots, X_m})$ norm, where the functions $\mathbb{E}_{X_1}\widehat{f}, \mathbb{E}_{X_1}f^*$ and the marginal probability distribution $P_{X_2, \dots, X_m}$ are defined on the rest of variables $\{X_2, \dots, X_m\}$, By Jensen's inequality, we infer that for any realization of $X_2=x_2, X_3=x_3, \dots, X_m=x_m$,
\begin{align*}
(\mathbb{E}_{X_1} \widehat{f}(X_1, x_2, \dots, x_m) & - \mathbb{E}_{X_1} f^*(X_1, x_2, \dots, x_m))^2 \\ & \leq \mathbb{E}_{X_1} [(\widehat{f}(X_1, x_2, \dots, x_m) - f^*(X_1, x_2, \dots, x_m))^2]
\end{align*}
Plugging it in the $\epsilon$-closeness assumption leads to,

$$ ||\mathbb{E}_{X_1}\widehat{f} - \mathbb{E}_{X_1}f^*||_{\mathcal{L}^2(P_{X_2, \dots, X_m})} \leq ||\widehat{f} - f^*||_{\mathcal{L}^2(P_{X_1, X_2, \dots, X_m})} \leq \epsilon, $$
which guarantees that $\mathbb{E}_{X_1}\widehat{f}$ is also $\epsilon$-closs to $\mathbb{E}_{X_1}f^*$ and hence it's a good estimator. In the sequel, a natural solution would be to estimate $\mathbb{E}_{X_1}\widehat{f}$ by taking averages of $\widehat{f}$ over different samples of $X_1$. However, for the linear regression problem that the estimator has a linear structure of the input, it is straightforward to show that it is enough to evaluate $\widehat{f}$ at $\mathbb{E} [X_1]$. And finally due to the zero-centering step of data preprocessing, $\mathbb{E} [X_1] = 0$. Thus, the aforementioned procedure is equivalent to zero-masking.

\section{A Note on the Number of Partitions} \label{app:k}
The number of partitions $k$ affects the performance of our algorithm in practice since a larger number of partitions will help in removing a bias in the estimates. However, in our experiments, we observe that a small number of partitions is sufficient to achieve good results. Furthermore, an excessive number of random partitions may have a detrimental effect, due to the possible small number of samples in each partition. Hence, we believe that the number of partitions will not drastically affect performance in practice. Reasonable choices of $k$ for our experiments range between 3-7, hence $k = \mathcal{O}(1)$ w.r.t. parameters of the problem. Thus, the resulting runtime can be reported as $\mathcal{O}(md)$.

\section{Computational Complexity and Comparison}
\label{app:comp}

As discussed in~\cref{sec:related_work}, compared to SITD, conditional independence-based approaches such as PCMCI~\citep{runge2019detecting}, PCMCI+~\citep{runge2020discovering}, and LPCMCI~\citep{gerhardus2020high} face exponential computational barriers. It is widely known that even endowed with a perfect infinite sample independence testing oracle, learning Bayesian Networks becomes NP-Hard~\citep{chickering2004large,chickering1996learning}. Consequently, computational challenges arise not only due to the nature of the conditional independence tests themselves but also from the computational intractability of searching through the exponentially large space of possible network structures. Hence, the runtime of the $\mathcal{O}(m)$ number of regressions that SITD demands is negligible compared to the exponential number of conditional independence tests from lengthy time-series. To support this argument in practice, we provide a runtime comparison between SITD and PCMCI+ w.r.t. the number of nodes $m$ in Table \ref{table:runtime_PCMCI}.

\begin{table}[ht]
\centering
\resizebox{\textwidth}{!}{
\begin{tabular}{lcccccccc}
      \toprule
       & 10 & 20 & 30 & 40 & 50 & 100 & 200 & 400\\
      \midrule
      SITD  &  $42 \pm 13$ & $35 \pm 6$ & $29 \pm 1$ & $30 \pm 4$ & $35 \pm 15$ & $41 \pm 6$ & $62 \pm 6$& $77 \pm 10 $\\
      PCMCI+& $4.2 \pm 0.4$ & $18.6 \pm 0.8$ & $48.6 \pm 1.4$ & $99.2 \pm 10$ & $216.4 \pm 42.2$ & $1091 \pm 65$ & $5678 \pm 264 $ & $\approx 8$ hours\\
      \bottomrule
  \end{tabular}}
  \captionof{table}{Table with runtime means and standard deviations for SITD and PCMCI+ (in seconds).
  \label{table:runtime_PCMCI}}
\end{table} 
%
%\newpage
\section{Additional Experiments}
\label{sec:appendix_experiments}
\subsection{Synthetic Experiments}
\label{sec:missing_table}
%For each experiment with synthetically generated data we use the following procedure to create the dataset:
%
\paragraph{Dataset generation.} We first set the number of potential causes $m$, and we fix the lag $\Delta$ and the number of time steps for the dataset $T$. We create a covariate adjacency 3-dimensional tensor $\Sigma$ of dimensions $\Delta \times m \times m$. This tensor has $0$-$1$ coefficients, where $\Sigma_{k,i,j} = 1$ if $X^i_{t - k}$ has a casual effect on $X^j_{t}$ for all time steps $t$. Similarly, we create an adjacency matrix $\Sigma^{\boldsymbol{Y}}$ for the outcome $\boldsymbol{Y}$. $\Sigma^{\boldsymbol{Y}}$ is a binary $\Delta \times m $ array, such that $\Sigma^{\boldsymbol{Y}}_{k,j}=1$ if $X_{t-k}^{j}$ has a causal effect on $Y_{t}$ for all time steps $t$. The entries of $\Sigma$ and $\Sigma^{\boldsymbol{Y}}$ follow the Bernouli distribution with parameter $p=0.5$. Note that the resulting casual structure fulfills \ref{cond:2}-\ref{cond:11}. 

We then create $m$ transformations that are used to produce the potential causes $\boldsymbol{X}^1, \dots, \boldsymbol{X}^m$. Each one of these transformations is modeled by an \textsc{MLP} with $1$ hidden layer and $200$ hidden units. We use \textsc{Tanh} nonlinearities (included also in the output layer) in order to control the scale of the values. The final output value is further scaled up so that all transforms generate values in the range $[-10,10]$. The input layer of each MLP is coming from the corresponding causal parents of the corresponding time series, as calculated from $\Sigma$. 

In order to generate the potential causes $\boldsymbol{X}^i$, we use $\Sigma$ and the MLP transforms. The first value of each time series is randomly generated from a uniform distribution in $[-10,10]$. Then, each $\boldsymbol{X}^{i}$ is produced by applying the appropriate transform to its causal parents, as determined by $\Sigma$, and a zero-mean unit variance Gaussian noise is added. We generate the target time series in a similar fashion. Each variable $Y_{t}$ is produced by applying the MLP transform to its causal parents, as determined by the target adjacency matrix $\Sigma^{\boldsymbol{Y}}$. We then add zero-mean Gaussian noise. The scale of the posterior additive noise for the outcome is referred to as the \emph{noise-to-signal ratio} (NTS).

\paragraph{Description of the experiments.} We are given a dataset as described above with $m$ potential causes and a fixed NTS for the generation of the outcome $\boldsymbol{Y}$. We determine which series $\boldsymbol{X}^1, \dots, \boldsymbol{X}^n$ are the causal parents of the outcome, using Algorithm \ref{alg}. For a given choice of $m$ and NTS, we repeat the experiments five times, and we report on the sample mean for the Accuracy (see Table \ref{table:snthetic1}). We additionally report on the F1 Score and CSI Score in Table \ref{table:snthetic2}-\ref{table:snthetic3} in the Appendix. This experiment is repeated for an increasing number of potential causes, and increasing noise-to-signal ratio, to evaluate the performance of Algorithm \ref{alg} on challenging datasets.

In this set of experiments, we learn $\eta_j^i$ as in Line \ref{alg:regression} of Algorithm \ref{alg}, using for the regression task an MLP model. We found that this simple approach, combined with zero-masking, dramatically reduces the false positives of the Student's t-test in Line \ref{alg:test} of Algorithm \ref{alg}.

\paragraph{Results.} Table \ref{table:snthetic1} shows the performance of our method with respect to the accuracy, for an increasing number of potential causes and increasing NSR. We observe that our method maintains a good score. These results are partially confirmed when we look at the F1 and CSI scores (see Table \ref{table:snthetic2}-\ref{table:snthetic3} in the Appendix). In fact, we see that the \alg is stable for an increasingly higher posterior noise. 

\begin{figure}[t]
    \centering
    \includegraphics[width=6in]
    {only_auroc.png}
    \caption{AUROC metric for RHINO and SITD for various noise levels on the synthetic dataset.}
    \label{AUROC_synthetic_dataset}
\end{figure}

In Figure~\ref{AUROC_synthetic_dataset} we plot the AUROC performance of SITD against RHINO on the synthetic dataset, confirming the competitive performance of STID. In order to calculate the AUROC for SITD, we sort our predictions (for existence of an edge)  on
   the 
   standard deviation of 
   $Z:= Y_T \cdot \tilde{g}_j^i + \tilde{\alpha}_j^i \cdot (Y_T - \tilde{g}_j^i ) - Y_T \cdot g_j^0 - \alpha_j^0 \cdot (Y_T - g_j^0 )$, which is simply the difference of the doubly robust statistics for $\theta^i$ and $\theta^0$ for a datapoint in partition $D_j$. 

%

%\improve{ Moreover, on this synthetic dataset, we compare against RHINO using the AUROC metric (shown in Appendix \ref{sec:AUROC_synthetic_exp}), confirming the competitive performance of SITD.}% \improve{Anything else that you would like to add here?}

\begin{table}[t]
  \centering
  %\vspace{-3mm}
  \caption{Accuracy of our method for increasing number of potential causes $m$, and different noise-to-signal ration (\textsc{NSR}). We observe that our method maintains good accuracy, even in challenging settings with many potential causes and high noise.}
  \label{table:snthetic1}
{\scriptsize
\begin{tabular}{lccccccc}%{|l|c|c|c|c|c|c|c|}
\toprule
   & \multicolumn{7}{c}{\textbf{Accuracy}} \\
\cmidrule(lr){2-8}
$\boldsymbol{\feat}$   & $\boldsymbol{\nsr=0}$            &$\boldsymbol{\nsr=0.05}$        & $\boldsymbol{\nsr=0.1}$          &$\boldsymbol{\nsr=0.15}$        &$\boldsymbol{\nsr=0.2}$         &$\boldsymbol{\nsr=0.25}$        & $\boldsymbol{\nsr=0.3}$         \\
\hline
       $\boldsymbol{5}$ & 0.60 $\pm$ 0.09 & 0.74 $\pm$ 0.25 & 0.66 $\pm$ 0.19 & 0.90 $\pm$ 0.11 & 0.80 $\pm$ 0.06 & 0.82 $\pm$ 0.10 & 0.94 $\pm$ 0.12 \\
       $\boldsymbol{10}$& 0.99 $\pm$ 0.02 & 0.92 $\pm$ 0.08 & 0.97 $\pm$ 0.04 & 0.79 $\pm$ 0.18 & 0.89 $\pm$ 0.06 & 0.94 $\pm$ 0.04 & 0.90 $\pm$ 0.08 \\
       $\boldsymbol{15}$& 0.89 $\pm$ 0.05 & 0.89 $\pm$ 0.05 & 0.88 $\pm$ 0.10 & 0.85 $\pm$ 0.02 & 0.79 $\pm$ 0.11 & 0.79 $\pm$ 0.09 & 0.81 $\pm$ 0.03 \\
       $\boldsymbol{20}$& 0.83 $\pm$ 0.07 & 0.73 $\pm$ 0.05 & 0.72 $\pm$ 0.07 & 0.77 $\pm$ 0.10 & 0.73 $\pm$ 0.05 & 0.75 $\pm$ 0.05 & 0.69 $\pm$ 0.06 \\
       $\boldsymbol{25}$& 0.76 $\pm$ 0.04 & 0.72 $\pm$ 0.10 & 0.71 $\pm$ 0.06 & 0.63 $\pm$ 0.08 & 0.68 $\pm$ 0.04 & 0.71 $\pm$ 0.07 & 0.66 $\pm$ 0.04 \\
       $\boldsymbol{30}$ & 0.76 $\pm$ 0.04 & 0.74 $\pm$ 0.04 & 0.72 $\pm$ 0.07 & 0.70 $\pm$ 0.10 & 0.66 $\pm$ 0.05 & 0.68 $\pm$ 0.04 & 0.64 $\pm$ 0.07 \\
       $\boldsymbol{35}$& 0.68 $\pm$ 0.02 & 0.65 $\pm$ 0.07 & 0.72 $\pm$ 0.06 & 0.65 $\pm$ 0.03 & 0.66 $\pm$ 0.05 & 0.61 $\pm$ 0.07 & 0.64 $\pm$ 0.09 \\
       $\boldsymbol{40}$ & 0.64 $\pm$ 0.03 & 0.69 $\pm$ 0.05 & 0.67 $\pm$ 0.05 & 0.62 $\pm$ 0.03 & 0.63 $\pm$ 0.06 & 0.58 $\pm$ 0.07 & 0.60 $\pm$ 0.07 \\
       $\boldsymbol{45}$ & 0.65 $\pm$ 0.04 & 0.68 $\pm$ 0.08 & 0.58 $\pm$ 0.04 & 0.61 $\pm$ 0.03 & 0.64 $\pm$ 0.04 & 0.59 $\pm$ 0.04 & 0.61 $\pm$ 0.06 \\
       $\boldsymbol{50}$ & 0.68 $\pm$ 0.05 & 0.63 $\pm$ 0.05 & 0.64 $\pm$ 0.06 & 0.63 $\pm$ 0.05 & 0.66 $\pm$ 0.05 & 0.59 $\pm$ 0.08 & 0.64 $\pm$ 0.07 \\
\bottomrule
\end{tabular}
}
\end{table}

%

%
%
%
%
%\subsubsection{Missing Tables of Section \ref{sec:missing_table}}
%
We provide the CSI Score in Table \ref{table:snthetic3} and the F1 Score in Table \ref{table:snthetic2} for the experiments on synthetic datasets. Recall that in this set of experiments we considered synthetic datasets with varying numbers of potential causes ($m$) and noise-to-signal ratio (NSR). Increasing $m$ and NSR give more challenging settings. We observe that our method maintains good CSI and F1 scores, for increasing NSR. 
\begin{table}[ht]
  \centering
  %\vspace{-3mm}
  \caption{CSI Score of Algorithm \ref{alg} for increasing number of potential causes $m$, and different noise-to-signal ration (\textsc{NSR}). Again, we observe that our method is robust to increasing \textsc{NSR}.}
  \label{table:snthetic3}
{\scriptsize
\begin{tabular}{lccccccc}%{|l|c|c|c|c|c|c|c|}
\toprule
   & \multicolumn{7}{c}{\textbf{CSI Score}} \\
\cmidrule(lr){2-8}
$\boldsymbol{\feat}$    & $\boldsymbol{\nsr=0}$            &$\boldsymbol{\nsr=0.05}$        & $\boldsymbol{\nsr=0.1}$          &$\boldsymbol{\nsr=0.15}$        &$\boldsymbol{\nsr=0.2}$         &$\boldsymbol{\nsr=0.25}$        & $\boldsymbol{\nsr=0.3}$         \\
\hline
      $\boldsymbol{5}$ & 0.57 $\pm$ 0.07 & 0.71 $\pm$ 0.28 & 0.63 $\pm$ 0.19 & 0.86 $\pm$ 0.12 & 0.69 $\pm$ 0.10 & 0.73 $\pm$ 0.12 & 0.91 $\pm$ 0.17 \\
    $\boldsymbol{10}$ & 0.98 $\pm$ 0.04 & 0.86 $\pm$ 0.14 & 0.95 $\pm$ 0.06 & 0.69 $\pm$ 0.21 & 0.80 $\pm$ 0.09 & 0.87 $\pm$ 0.07 & 0.82 $\pm$ 0.14 \\
    $\boldsymbol{15}$ & 0.80 $\pm$ 0.07 & 0.77 $\pm$ 0.11 & 0.75 $\pm$ 0.16 & 0.68 $\pm$ 0.06 & 0.59 $\pm$ 0.19 & 0.57 $\pm$ 0.15 & 0.59 $\pm$ 0.03 \\
     $\boldsymbol{20}$ & 0.66 $\pm$ 0.12 & 0.52 $\pm$ 0.12 & 0.46 $\pm$ 0.07 & 0.56 $\pm$ 0.10 & 0.46 $\pm$ 0.08 & 0.51 $\pm$ 0.07 & 0.39 $\pm$ 0.09 \\
     $\boldsymbol{25}$ & 0.51 $\pm$ 0.06 & 0.45 $\pm$ 0.12 & 0.43 $\pm$ 0.09 & 0.37 $\pm$ 0.09 & 0.38 $\pm$ 0.05 & 0.41 $\pm$ 0.08 & 0.33 $\pm$ 0.06 \\
     $\boldsymbol{30}$  & 0.47 $\pm$ 0.05 & 0.50 $\pm$ 0.07 & 0.46 $\pm$ 0.12 & 0.38 $\pm$ 0.08 & 0.35 $\pm$ 0.08 & 0.34 $\pm$ 0.05 & 0.31 $\pm$ 0.07 \\
     $\boldsymbol{35}$  & 0.42 $\pm$ 0.04 & 0.31 $\pm$ 0.06 & 0.39 $\pm$ 0.07 & 0.29 $\pm$ 0.07 & 0.30 $\pm$ 0.09 & 0.22 $\pm$ 0.09 & 0.26 $\pm$ 0.09 \\
     $\boldsymbol{40}$  & 0.32 $\pm$ 0.06 & 0.38 $\pm$ 0.05 & 0.33 $\pm$ 0.08 & 0.29 $\pm$ 0.06 & 0.24 $\pm$ 0.06 & 0.20 $\pm$ 0.07 & 0.19 $\pm$ 0.11 \\
     $\boldsymbol{45}$  & 0.33 $\pm$ 0.10 & 0.34 $\pm$ 0.07 & 0.20 $\pm$ 0.02 & 0.22 $\pm$ 0.05 & 0.25 $\pm$ 0.03 & 0.20 $\pm$ 0.05 & 0.19 $\pm$ 0.06 \\
     $\boldsymbol{50}$ & 0.33 $\pm$ 0.03 & 0.29 $\pm$ 0.06 & 0.29 $\pm$ 0.06 & 0.23 $\pm$ 0.04 & 0.26 $\pm$ 0.06 & 0.21 $\pm$ 0.08 & 0.26 $\pm$ 0.07 \\
\bottomrule
\end{tabular}
}
\end{table}
\begin{table}[t]
  \centering
  \caption{F1 Score of the \alg for increasing number of potential causes $m$, and different noise-to-signal ration (\textsc{NSR}). Interestingly, our method maintains a good F1 score for increasing \textsc{NSR}.}
  \label{table:snthetic2}
{\scriptsize
\begin{tabular}{lccccccc}%{|l|c|c|c|c|c|c|c|}
\toprule
   & \multicolumn{7}{c}{\textbf{F1 Score}} \\
\cmidrule(lr){2-8}
$\boldsymbol{\feat}$ & $\boldsymbol{\nsr=0}$            &$\boldsymbol{\nsr=0.05}$        & $\boldsymbol{\nsr=0.1}$          &$\boldsymbol{\nsr=0.15}$        &$\boldsymbol{\nsr=0.2}$         &$\boldsymbol{\nsr=0.25}$        & $\boldsymbol{\nsr=0.3}$         \\
\hline
       $\boldsymbol{5}$ & 0.73 $\pm$ 0.06 & 0.79 $\pm$ 0.20 & 0.75 $\pm$ 0.12 & 0.92 $\pm$ 0.07 & 0.81 $\pm$ 0.07 & 0.84 $\pm$ 0.08 & 0.95 $\pm$ 0.11 \\
       $\boldsymbol{10}$ & 0.99 $\pm$ 0.02 & 0.92 $\pm$ 0.09 & 0.98 $\pm$ 0.03 & 0.80 $\pm$ 0.15 & 0.89 $\pm$ 0.06 & 0.93 $\pm$ 0.04 & 0.90 $\pm$ 0.09 \\
       $\boldsymbol{15}$ & 0.89 $\pm$ 0.05 & 0.86 $\pm$ 0.08 & 0.85 $\pm$ 0.11 & 0.81 $\pm$ 0.04 & 0.73 $\pm$ 0.15 & 0.72 $\pm$ 0.12 & 0.74 $\pm$ 0.03 \\
       $\boldsymbol{20}$ & 0.79 $\pm$ 0.08 & 0.67 $\pm$ 0.10 & 0.62 $\pm$ 0.07 & 0.71 $\pm$ 0.09 & 0.63 $\pm$ 0.07 & 0.67 $\pm$ 0.06 & 0.56 $\pm$ 0.09 \\
       $\boldsymbol{25}$ & 0.68 $\pm$ 0.05 & 0.61 $\pm$ 0.11 & 0.60 $\pm$ 0.09 & 0.53 $\pm$ 0.11 & 0.55 $\pm$ 0.05 & 0.57 $\pm$ 0.08 & 0.49 $\pm$ 0.07 \\
       $\boldsymbol{30}$ & 0.64 $\pm$ 0.05 & 0.66 $\pm$ 0.06 & 0.62 $\pm$ 0.10 & 0.54 $\pm$ 0.09 & 0.51 $\pm$ 0.09 & 0.50 $\pm$ 0.06 & 0.46 $\pm$ 0.09 \\
       $\boldsymbol{35}$ & 0.59 $\pm$ 0.05 & 0.47 $\pm$ 0.07 & 0.56 $\pm$ 0.07 & 0.45 $\pm$ 0.08 & 0.46 $\pm$ 0.11 & 0.35 $\pm$ 0.11 & 0.41 $\pm$ 0.11 \\
       $\boldsymbol{40}$ & 0.49 $\pm$ 0.07 & 0.55 $\pm$ 0.05 & 0.49 $\pm$ 0.08 & 0.45 $\pm$ 0.07 & 0.38 $\pm$ 0.08 & 0.33 $\pm$ 0.09 & 0.30 $\pm$ 0.15 \\
       $\boldsymbol{45}$ & 0.49 $\pm$ 0.11 & 0.50 $\pm$ 0.08 & 0.34 $\pm$ 0.03 & 0.36 $\pm$ 0.06 & 0.40 $\pm$ 0.04 & 0.33 $\pm$ 0.06 & 0.32 $\pm$ 0.08 \\
       $\boldsymbol{50}$ & 0.50 $\pm$ 0.03 & 0.44 $\pm$ 0.07 & 0.44 $\pm$ 0.08 & 0.38 $\pm$ 0.05 & 0.41 $\pm$ 0.07 & 0.34 $\pm$ 0.11 & 0.40 $\pm$ 0.09 \\
\bottomrule
\end{tabular}
}
\end{table}

%\subsubsection{Comparison on synthetic dataset}\label{sec:AUROC_synthetic_exp}
\newpage
\if{0}
\begin{figure}[t]
    \centering
    \includegraphics[width=5in]
    {figs/only_auroc.png}
    \caption{AUROC metric for RHINO and SITD for various noise levels on the synthetic dataset.}
    \label{AUROC_synthetic_dataset}
\end{figure}
\fi

%In Figure~\ref{AUROC_synthetic_dataset} we plot the AUROC performance of SITD against RHINO on the synthetic dataset. In order to calculate the AUROC for SITD, we sort our predictions (for existence of an edge)  on the standard deviation of 
  % $Z:= Y_T \cdot \tilde{g}_j^i + \tilde{\alpha}_j^i \cdot (Y_T - \tilde{g}_j^i ) - Y_T \cdot g_j^0 - \alpha_j^0 \cdot (Y_T - g_j^0 )$, which is simply the difference of the doubly robust statistics for $\theta^i$ and $\theta^0$ for a datapoint in partition $D_j$. 

\subsection{Performance in Low-Sample Regimes}
\label{sec:low_sample}
Here we report the results for additional experiments in the practically important low sample setting.  In~\Cref{fig:exp_observations}, the plots are provided to support~\Cref{sec:addexp}. The double robustness property enables our algorithm to rely on simple estimators with low statistical complexity. As a result, our method shows more consistent performance in low-sample regimes as opposed to existing approaches that are based on overparameterized models demanding so many data points.

\begin{figure}[h!]
    \centering
    \begin{subfigure}[t]{2.7in}
        \centering
        \includegraphics[width=2.7in]{Ecoli1.png}
        \caption{Task: E.Coli 1}\label{fig:1a}        
    \end{subfigure}
    \begin{subfigure}[t]{2.7in}
        \centering
        \includegraphics[width=2.7in]{Ecoli2.png}
        \caption{Task: E.Coli 2}\label{fig:1b}    
   \end{subfigure}
   \begin{subfigure}[t]{2.7in}
        \centering
        \includegraphics[width=2.7in]{Yeast1.png}
        \caption{Task: Yeast 1}\label{fig:1c}    
   \end{subfigure}
   \begin{subfigure}[t]{2.7in}
        \centering
        \includegraphics[width=2.7in]{Yeast2.png}
        \caption{Task: Yeast 2}\label{fig:1d}    
    \end{subfigure}
    \begin{subfigure}[t]{2.7in}
        \centering
        \includegraphics[width=2.7in]{Yeast3.png}
        \caption{Task: Yeast 3}\label{fig:1e}    
    \end{subfigure}
    \caption{This figure demonstrates the consistent performance of SITD w.r.t number of observations compared to state-of-the-art methods Rhino and Rhino+g. Note that Rhino and Rhino+g are built on neural networks. SITD significantly outperforms Rhino and Rhino+g in E.Coli 1 and E.Coli 2 and shows competitive results in Yeast 1. 
    Thanks to the double robustness property of SITD, the dependence of our algorithm on the estimator is much lower than the well-established approaches. In this regard, SITD with a simple kernel regression with polynomial kernels has superior performance compared to state-of-the-art methods Rhino and Rhino+g. This superiority gets magnified in the low number of observation regimes due to the high sample complexity required by Rhino and Rhino+g.}\label{fig:exp_observations}
\end{figure}

\subsection{Run Time and Hardware}
\label{app:runtime}
\begin{table}[h]
\centering
\caption{Run time and Hardware used for our method (SITD) and the state-of-the-art baseline Rhino.}
{\scriptsize
\begin{tabular}{l c c}
\toprule
\textbf{Category\textbackslash Method}  & \textbf{Rhino} & \textbf{SITD (ours)} \\
\midrule
Runtime  & 18 mins 40 sec $\pm$ 30 sec & 57.12 sec $\pm$ 1.6 sec \\    
\midrule
Hardware & 1 NVIDIA A100 GPU + AMD EPYC 7402 24-Core CPU & 11th Gen Core i5-1140F CPU \\
\bottomrule
\end{tabular}
}
\label{table:runtime}
\end{table} 

To give a taste of the computational efficiency of our method, here we report the average runtime of SITD and the competitive rival Rhino for experiment~\cref{table: Exp DREAM3 AUROC} across all five tasks (E.Coli 1, E.Coli 2, Yeast 1, Yeast 2 and Yeast 3) in~\Cref{table:runtime}. Despite having access only to a single CPU in contrast to the GPU-equipped execution of Rhino our method is almost 20x faster. This is because of the fact that SITD algorithm will provide reasonable results even when employing simple fast efficient estimators (in this case a kernel regression).
